# Supplementary material for: Tensor Convolutional Network for Higher-Order Interaction Prediction in Sparse Tensors
Source: arXiv:2503.11786 source file (2025-03-14)
Supplement: Supplementary file 1 [file 080appendix.tex]

\begin{table} [h]
	\centering
	\caption{Symbol description.}
	\label{tab:notation}
%	\footnotesize
	\resizebox{0.99\columnwidth}{!}{%
		\begin{tabular}{cl}
			\toprule
			\textbf{Symbol} & \textbf{Description} \\
			\midrule
			$\T{X}$ & (sparse) tensor \\
                $\mat{A}^{(n)}$ & $n$-th factor matrix \\
                $\mat{F}^{[0]}$ & concatenation of factor matrices $\mat{A}^{(n)}$ \\
                $\mat{F}^{[l]}$ & output of $l$-th layer in \method \\
                $G_H$ & hypergraph originated from a sparse tensor $\T{X}$ \\
                $G_C$ & clique expanded graph from $G_H$ \\
                $\mat{B}$ & incidence matrix of $G_H$ \\
                $\mat{A}$ & adjacency matrix of $G_C$ \\                
			$\Omega_o$ & set of observed entries of a tensor $\T{X}$ \\
			$\Omega_u$ & set of unobserved entries of a tensor $\T{X}$ \\
   			$i_n$ & $i$-th entity of $n$-th dimension \\
			$(i_1,...,i_N)$ & interaction in a tensor \\
                $r$ & column size of factor matrices \\
                $|\cdot|$ & cardinality of a set \\
                $\|$ & horizontal concatenation \\
                $\vee$ & vertical concatenation \\
			\bottomrule
		\end{tabular}
	}
\end{table}

\section{Proofs of Complexities}
\label{subsec:appendix:complexities}

\begin{proof}
    The number of edges of a hypergraph is the same number of interactions of a sparse tensor.
    For a COO format, we need to store $N|E|$ indices for the hypergraph, and hence the space and time complexities are $O(N|E|)$.
\end{proof}

\begin{proof}
We start from computing the number of nonzeros in a $j$-th column of the matrix $\mathbf{A}$ (i.e., $\mathbf{A}[:,j]$).
We can obtain $\mathbf{A}[:,j]$ by computing $\mathbf{B}\times \mathbf{B}^T[:,j]$.
$\mathbf{A}[:,j]$ has at most $N\times n_j$ nonzeros where $n_j$ is the number of nonzeros in $\mathbf{B}^T[:,j]$.
This is because (1) we only consider the columns of $\mathbf{B}$ corresponding to the rows associated with nonzero elements in $\mathbf{B}^T[:,j]$, (2) $\mathbf{B}^T[:,j]$ has $n_j$ nonzeros, and (3) each column of $\mathbf{B}$ has $N$ nonzeros.
In other words, since each column of $\mathbf{B}$ can generate up to $N$ nonzeros in $\mathbf{A}[:,j]$, and we utilize $n_j$ columns of $\mathbf{B}$ to create nonzeros in $\mathbf{A}[:,j]$, the number of nonzeros in $\mathbf{A}[:,j]$ is at most $N\times n_j$.
Then, the space complexity of a matrix $\mathbf{A}$ is $O(\sum_{j=1}^{|V|}{N\times n_j}) = O(N\times (n_1 + ... + n_{|V|})) = O(N^2|E|)$ since $(n_1 + ... + n_{|V|})$ is equal to $N|E|$ which is the number of nonzeros in $\mathbf{B}^T$.
\end{proof}

\begin{proof}
The dominant computation in Equation~\eqref{eq:ceg} is $\mat{B}\mat{B}^T$.
As described in the space complexity, for computing $\mathbf{A}[:,j] = \mat{B}\mat{B}^T[:,j]$, we utilize (1) $\mathbf{B}^T[:,j]$ and (2) the $n_j$ columns of $\mathbf{B}$ corresponding to the rows associated with nonzero elements in $\mathbf{B}^T[:,j]$.
Note that $n_j$ is the number of nonzeros in $\mathbf{B}^T[:,j]$.
Let us denote the positions of the nonzeros in $\mathbf{B}^T[:,j]$ as $p_1,...,p_{n_j}$.
Then we construct the sub-matrix $\mathbf{B}_j \in \mathbb{R}^{|V|\times n_j}$ by selecting columns indexed by $p_1,...,p_{n_j}$ from matrix $\mat{B}$.
The resulting sub-matrix $\mathbf{B}_j$ has $N\times n_j$ non-zero entries.
Also, let a vector composed of the nonzero elements of $\mathbf{B}^T[:,j]$ be $\mathbf{b}_j \in \mathbb{R}^{n_j}$.
Then, the time complexity for $\mathbf{A}[:,j]$ is $O(N \times n_j)$ since sparse matrix-vector multiplication between the sub-matrix $\mathbf{B}_j$ and the vector $\mathbf{b}_j$ requires $O(N\times n_j)$ time.
Thus, the time complexity for $\mathbf{A}$ is $O(\sum_{j=1}^{|V|}{N\times n_j}) = O(N\times (n_1 + ... + n_{|V|})) = O(N^2|E|)$ since $(n_1 + ... + n_{|V|})$ is equal to $N|E|$ which is the number of nonzeros in $\mathbf{B}^T$.
\end{proof}

 \begin{figure*}[h]
 %	\vspace{-3mm}
 %\qquad\qquad\raggedright
 %	 \subfloat{\includegraphics[width=0.45\textwidth]{FIG/PERF/LEGEND.pdf}} \\
 %	\vspace{-3mm}	
 %	 \setcounter{subfigure}{0}
 	\centering	
 	 \subfloat[Degree distribution on ML-100k dataset]{\includegraphics[width=0.19\textwidth]{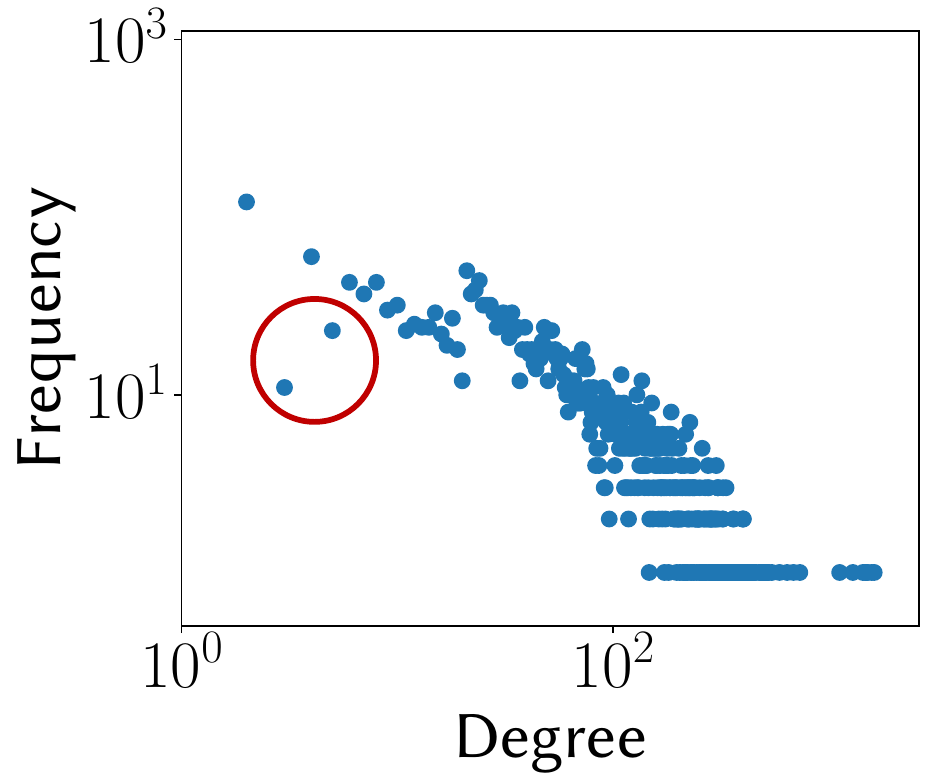}\label{fig:ml_ht}} 
 	 \subfloat[Degree distribution on SG dataset]{\includegraphics[width=0.19\textwidth]{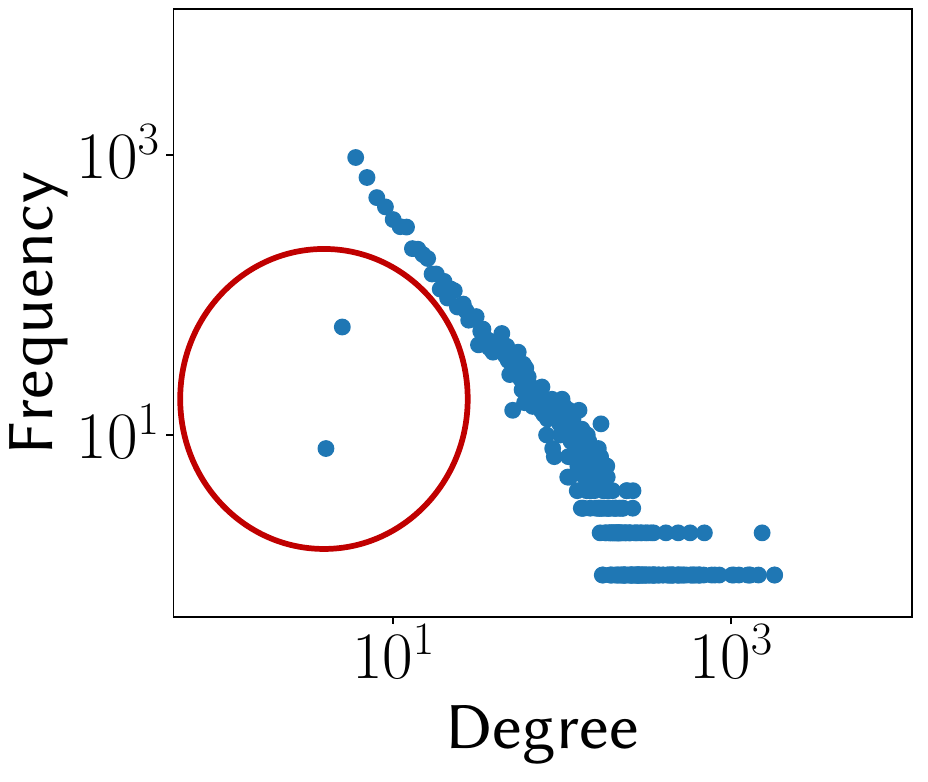}\label{fig:sg_ht}}
 	 \subfloat[Degree distribution on Gowalla dataset]{\includegraphics[width=0.19\textwidth]{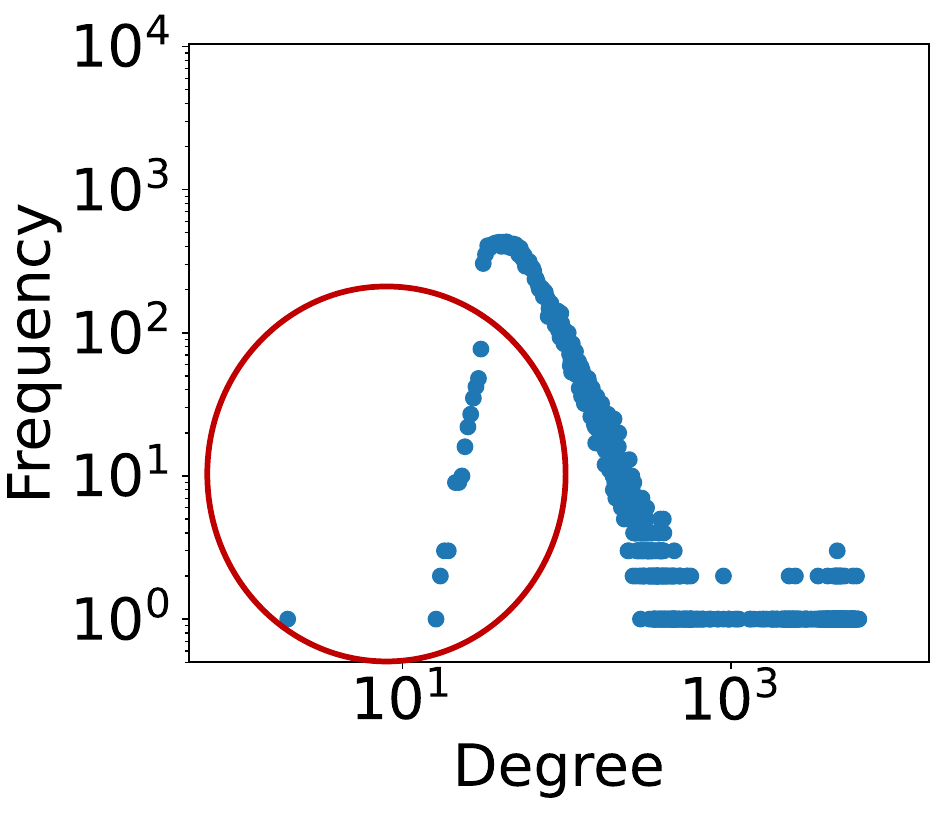}\label{fig:gowalla_ht}} 	 
 	 \subfloat[{Degree distribution on UCI dataset}]{\includegraphics[width=0.19\textwidth]{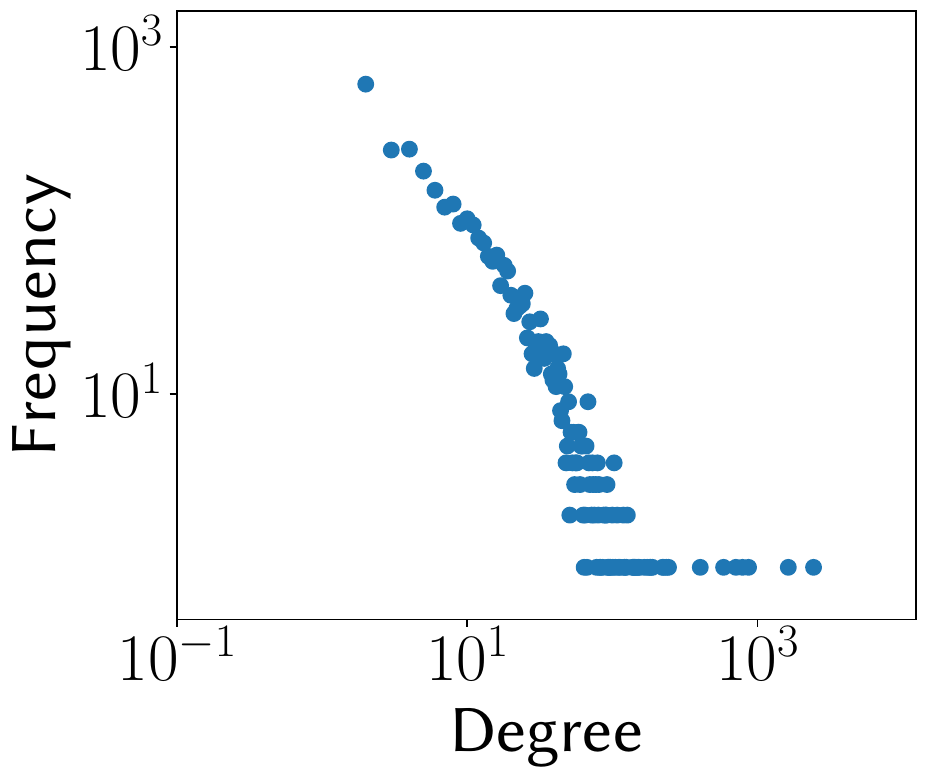}\label{fig:uci_ht}} 
 	 \subfloat[{Degree distribution on UMLS dataset}]{\includegraphics[width=0.19\textwidth]{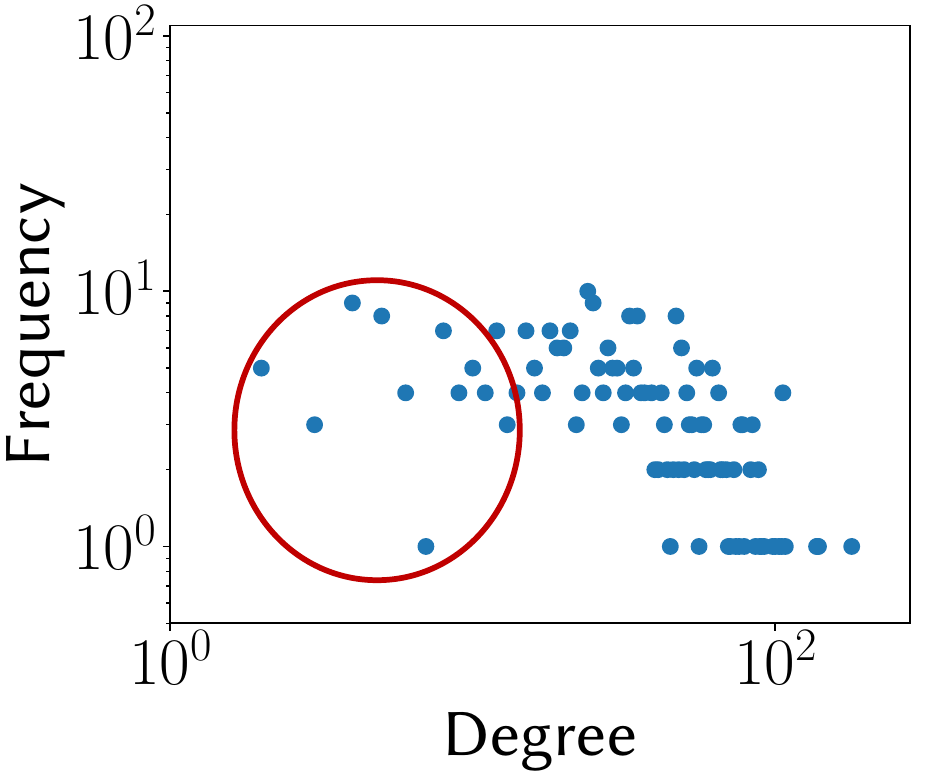}\label{fig:umls_ht}} \quad\quad	 	 
 	  \\
% 	 \subfloat[Singular value distribution on ML-100k dataset]{\includegraphics[width=0.19\textwidth]{FIG/PROPERTIES/ML_SV.pdf}\label{fig:ml_sv}}			 
% 	 \subfloat[Singular value distribution on SG dataset]{\includegraphics[width=0.19\textwidth]{FIG/PROPERTIES/SG_SV.pdf}\label{fig:sg_sv}}		
% 	 \subfloat[Singular value distribution on SG dataset]{\includegraphics[width=0.19\textwidth]{FIG/PROPERTIES/GOWALLA_SV.pdf}\label{fig:gowalla_sv}}		 	 
% 	 \subfloat[{Singular value distribution on UCI dataset}]{\includegraphics[width=0.19\textwidth]{FIG/PROPERTIES/UCI_SV.pdf}\label{fig:uci_sv}}		 	
% 	 \subfloat[{Singular value distribution on UMLS dataset}]{\includegraphics[width=0.19\textwidth]{FIG/PROPERTIES/UMLS_SV.pdf}\label{fig:umls_sv}}		 		 	 
% 	 	 \\
 	\caption{
 	Degree distribution of clique-expanded graph generated from sparse tensors.
 	}
 	\label{fig:characteristics}
 \end{figure*}

\begin{table*}[!h]
\caption{
Comparison of the performance of \method on 3rd-order and 4th-order tensors in ML-100k.
\method is more effective on the 4th-order tensor than the 3rd-order tensor in terms of the average improvement.
}
\label{tab:effectiveness_order}
\resizebox{0.99\textwidth}{!}{
\begin{tabular}{ll|rr|rr|rr|rr|rr|rr|r}
\toprule
\multicolumn{2}{c|}{Setting}                              & \multicolumn{2}{c|}{CP}                               & \multicolumn{2}{c|}{Tucker}                                   & \multicolumn{2}{c|}{NCFT} & \multicolumn{2}{c|}{M$^2$DMTF}   & \multicolumn{2}{c|}{NeAT}            & \multicolumn{2}{c|}{CostCo}                                   & \multicolumn{1}{c}{\multirow{2}{*}{\begin{tabular}[c]{@{}c@{}}Average\\ Improvement\end{tabular}}} \\
\multicolumn{1}{c}{Dataset} & \multicolumn{1}{c|}{Metric} & 
\multicolumn{1}{c}{w/o \method} & \multicolumn{1}{c|}{w/ \method} & 
\multicolumn{1}{c}{w/o \method} & \multicolumn{1}{c|}{w/ \method} & 
\multicolumn{1}{c}{w/o \method} & \multicolumn{1}{c|}{w/ \method} & 
\multicolumn{1}{c}{w/o \method} & \multicolumn{1}{c|}{w/ \method} & 
\multicolumn{1}{c}{w/o \method} & \multicolumn{1}{c|}{w/ \method} & 
\multicolumn{1}{c}{w/o \method} & \multicolumn{1}{c|}{w/ \method} & \multicolumn{1}{c}{}                                     \\
\midrule
\multirow{3}{*}{\begin{tabular}[c]{@{}c@{}}3rd-order tensor \\ (ML-100k)\end{tabular}}
& AP@100                      & 0.2548                 &       0.1646\blue{$\blacktriangledown$}                   & 0.2194                     & 0.2841\red{$\blacktriangle$}                           & 0.1972                   &         0.2523\red{$\blacktriangle$}              & 0.1976 & 0.2146\red{$\blacktriangle$} & 
0.1653 &  0.1695\red{$\blacktriangle$}  &
0.2749                     & \textbf{0.3105}\red{$\blacktriangle$}                          & 7.68\%                                                   \\
& AP@1000                     & 0.1746                 &       0.1308\blue{$\blacktriangledown$}                   & 0.1594                     & 0.1923\red{$\blacktriangle$}                           & 0.1688                   &        0.1956\red{$\blacktriangle$}                & 0.1389 & 0.1834\red{$\blacktriangle$} & 
 0.1262 &  0.1562\red{$\blacktriangle$}  &
0.1906                     & \textbf{0.2368}\red{$\blacktriangle$}                          & 15.24\%                                                  \\
& AP@10000                    & 0.0807                 &      0.0689\blue{$\blacktriangledown$}                 & 0.0766                     & 0.0928\red{$\blacktriangle$}                           & 0.0816                   &       0.0992\red{$\blacktriangle$}                  & 0.0650 & 0.0879\red{$\blacktriangle$} & 
0.0682 &  0.0869\red{$\blacktriangle$}  &
0.0956                     & \textbf{0.1179}\red{$\blacktriangle$}                          & 18.97\%     \\  
\midrule
\midrule
\multirow{3}{*}{\begin{tabular}[c]{@{}c@{}}4th-order tensor \\ (ML-100k)\end{tabular}} 
& AP@100                      & 0.0271                 &       0.0275\red{$\blacktriangle$}                   & 0.0566                     & 0.1309\red{$\blacktriangle$}                           & 0.0553                   &         0.1586\red{$\blacktriangle$}              & 0.0459 & 0.0943\red{$\blacktriangle$} & 
	0.0806 &  \textbf{0.2532} \red{$\blacktriangle$}    &
0.0845                     & 0.1309\red{$\blacktriangle$}                          & 115.6\%                                                   \\
& AP@1000                     & 0.0206                 &       0.0150\blue{$\blacktriangledown$}                   & 0.0355                     & 0.0705\red{$\blacktriangle$}                           & 0.0352                   &        0.1020\red{$\blacktriangle$}                & 0.0210 & 0.0568\red{$\blacktriangle$} &
	0.0401 & 0.0879 \red{$\blacktriangle$} &
 0.0509                     & \textbf{0.1048}\red{$\blacktriangle$}                          & 109.3\%                                                  \\
& AP@10000                    & 0.0101                 &      0.0071\blue{$\blacktriangledown$}                 & 0.0165                     & 0.0301\red{$\blacktriangle$}                           & 0.0162                   &       0.0392\red{$\blacktriangle$}                  & 0.0064 & 0.0218\red{$\blacktriangle$} &
	0.0176 & 0.0313 \red{$\blacktriangle$} &
 0.0255                     & \textbf{0.0521}\red{$\blacktriangle$}                          & 123.4\%     \\
\bottomrule
\end{tabular}}
\end{table*}

\section{Dataset}
\label{subsec:appendix:data}
ML-100k data is movie recommendation data of the form (user, movie, day, month).
SG data and Gowalla data are Point-of-interest (POI) recommendation data whose form is (user, location, time).
For Gowalla data, we filtered out entities (i.e., user, location, time) that have fewer than 30 interactions.
UCI data contains message-sending relationships between students at the University of California.
It has the form (sender, receiver, time).
UMLS is a medical knowledge graph of the form (subject, relation, object).
We randomly split observed interactions into train, validation, and test data with the ratio 7:1:2.

\section{Implementation Detail}
\label{appendix:sec:implementation_detail}
We describe the implementation details of competitors used in this paper.

\textbf{CP and Tucker decomposition.}
We implement gradient-based CP and Tucker decomposition methods using PyTorch.

\textbf{NCF extension for tensor (NCFT).}
We extend NCF~\cite{he2017neural} which mainly consists of matrix factorization and MLP layers.
We replace matrix factorization with CP decomposition and use $\|_{n=1}^{N} (\mat{A}^{(n)}(i_n,:)) \in \mathbb{R}^{Nr}$ as an input of MLP layers.

\textbf{CostCo.}
Since the paper~\cite{liu2019costco} provides the TensorFlow code on GitHub\footnote{\url{https://github.com/USC-Melady/KDD19-CoSTCo}}, we implement the code using PyTorch.
We use two types of convolution operation layers as proposed in the paper and a $2$-layer MLP predictor with the ReLU function.

\textbf{M$^2$DMTF.}
Since the paper~\cite{fan2021multi} provides the MATLAB code on GitHub\footnote{\url{https://github.com/jicongfan/Multi-Mode-Deep-Matrix-and-Tensor-Factorization}}, we implement the code using PyTorch.
We use a $2$-layer MLP (Multi-layer Perceptron) with the ReLU function for encoding factor matrices $\mat{A}^{(n)}$.

\textbf{NeAT.}
We implement the code using PyTorch and set hyperparameters (e.g., number of layers, dropout rate) referring to the code on GitHub\footnote{\url{https://anonymous.4open.science/r/NEAT/README.md}}.

\textbf{MLP.}
We use a $3$-layer MLP (Multi-layer Perceptron) predictor with the ReLU function.
Its input is $\|_{n=1}^{N} (\mat{A}^{(n)}(i_n,:)) \in \mathbb{R}^{Nr}$ for the interaction $(i_1,...,i_N)$.

\textbf{HyperConv.}
We first obtain the matrix $\mat{F}_{\textrm{hyper}} \in \mathbb{R}^{(I_1+\cdots+I_N)\times r}$ by propagating $\mat{F}^{[0]} \in \mathbb{R}^{(I_1+\cdots+I_N)\times r}$ over a tensor-originated hypergraph using HyperConv~\cite{bai2021hypergraph}.
We then predict a score using a $2$-layer MLP predictor where its input is $(\mat{A}^{(1)}(i_1,:) + \mat{A}_{\textrm{hyper}}^{(1)}(i_1,:)) * \cdots * (\mat{A}^{(N)}(i_N,:) + \mat{A}_{\textrm{hyper}}^{(N)}(i_N,:)) $ for the interaction $(i_1,...,i_N)$.
$*$ operation indicates element-wise product.
Note that we divide $\mat{F}_{\textrm{hyper}}$ into $N$ parts to obtain $\mat{A}_{\textrm{hyper}}^{(n)} \in \mathbb{R}^{I_n \times r}$ whose row indices correspond to those of $\mat{A}^{(n)}$.

\section{Metrics}
\label{subsec:appendix:metric}
We evaluate the performance in terms of two metrics: AP@$k$.
As described in Section~\ref{sec:experim}, AP@$k$ considers the number of test interactions and ranks of them in top-$k$ interactions.

\begin{itemize}
	\item Precision@k
	\begin{align}
		Precision@K = \frac{|\Omega_{prediction,k} \cap \Omega_{test}|}{k}
	\end{align}
	where $\Omega_{test}$ is a testset and $\Omega_{prediction,k}$ is a set of top-$k$ predicted interactions.
	\item AP@k (Average Precision@k)
	\begin{align}
		AP@k = \frac{1}{min(k, |\Omega_{test}|)} \sum_{i=1}^{k}{\text{Precision@i} * rel(i)}
	\end{align}
	where $rel(i) = \begin{cases}
  1 & \text{if $i$-th ranked interaction is in $\Omega_{test}$} \\
  0 & \text{otherwise}
\end{cases}$
% \begin{align}
% rel(i) = \begin{cases}
%   1 & \text{if $i$-th ranked entry is in $\Omega_{test}$} \\
%   0 & \text{otherwise}
% \end{cases}		
% 	\end{align}
\end{itemize}

\section{Effectiveness of \method on 3rd-order and 4th-order Tensors in ML-100k}
We compare the effectiveness of \method by varying the order of tensors in ML-100k: 3rd-order tensor and 4th-order tensor.
We use the 4th-order tensor in Table~\ref{tab:Description} and construct a 3rd-order tensor where its form is (user, movie, month), its size is $943\times 1663 \times 8$, and the number of observations is $999,811$.
Compared to the 4th-order tensor (See Table~\ref{tab:Description}), this 3rd-order tensor has some missing observations and items during the preprocessing stage. However, this does not significantly affect the comparison between the two tensors.

Table~\ref{tab:effectiveness_order} shows that \method is more effective on the 4th-order tensor than the 3rd-order tensor in terms of the average improvement.
This performance gap of the average improvement is because \method works effectively on highly sparse tensors as described in Sections~\ref{subsec:compatibility} and~\ref{subsec:performance}.
Note that the 4th-order tensor is more sparse than the 3rd-order tensor.
For the 4th-order tensor, due to its high sparsity, existing tensor factorization methods fail to effectively learn latent vectors of entities that have only a small number of interactions.
\method helps learn expressive latent vectors of entities, universally improving the performance of existing tensor factorization methods on the 4th-order tensor.

\section{Characteristics of Clique-Expanded Graphs (Q5)}
\label{appendix:sec:characteristics}
We investigate the degree distribution and singular value distribution of clique-expanded graphs obtained from sparse tensors.
As shown in Figure~\ref{fig:characteristics}, all data almost follows a heavy-tailed distribution.
Compared to real-world graphs, the frequencies of low-degree nodes (in red circle) are relatively low on ML-100k, SG, Gowalla, and UMLS datasets since there is no edge that does not form a clique in our graph; exceptionally, since UCI data is a temporal graph, it follows a heavy-tailed distribution better.
As tensor-originated graphs have similar characteristics to real-world graphs,
propagating information through these graphs works effectively, as shown in Section~\ref{subsec:ablation}, where various GNNs enhance the performance of tensor factorization.
